# Supplementary material for: Network Robustness via Global k-cores
Source: arXiv:2012.10036 source file (2020-12-18)
Supplement: Supplementary file 1 [file Appendix.tex]

\clearpage
\section{Supplementary}

\subsection{Parameterized Complexity}\label{subsec:pc}

In parameterized
complexity, each problem instance comes
with a parameter $p$. Formally, a parameterized problem $\Pi$ is a
subset of $\Gamma^{*}\times
\mathbb{N}$, where $\Gamma$ is a finite alphabet. An instance of a
parameterized problem is a tuple $(x,p)$, where $p$ is the
parameter. A central notion is \emph{fixed parameter
	tractability} (FPT) which means, for a
given instance $(x,p)$, solvability in time $f(k) \cdot poly(|x|)$,
where $f$ is an arbitrary computable function of $k$ and
$poly$ is a polynomial in the input size $|x|$.
We use the notation $\OO^*(f(p))$ to denote $O(f(p)poly(|x|))$. While there have been important examples of traditional algorithms that have been analyzed in this fashion, the theoretical foundations for deliberate design of such algorithms, and a complementary complexity-theoretic framework for hardness, were developed in the late nineties~\cite{DF95a,DF95b,ADF95,DF88,DowneyF99}.
Just as NP-hardness is used as an evidence that a problem is unlikely to be polynomial time solvable, there exists a hierarchy of complexity classes above FPT, and showing that a parameterized problem is hard for one of these classes is considered
evidence that the problem is unlikely to be fixed-parameter tractable. Indeed, assuming the Exponential Time Hypothesis~\cite{DBLP:journals/jcss/ImpagliazzoP01}, a problem that is hard for~\WO{} does not belong to \FPT{}. The main classes in this hierarchy are:

$ \FPT  \subseteq \WO \subseteq \WT \subseteq \cdots \subseteq \WP \subseteq \XP,$

\noindent where a parameterized problem belongs to the class \ensuremath{\mathsf{XP}} if there exists an algorithm for it with running time bounded by$|x|^{g(p)}$, where $g$ is an arbitrary computable function of $p$. For the hardness results, we will rely on parameterized reductions from known hard problems. The notion of parameterized reduction is defined as follows.

\begin{definition}
	Let $A,B$ be parameterized problems.  We say that $A$ is {\bf \em fpt-reducible} to $B$ if there exist functions
	$f,g:\mathbb{N}\rightarrow \mathbb{N}$, a constant $\alpha \in \mathbb{N}$, and
	an algorithm $\Phi$ which transforms an instance $(x,p)$ of $A$ into an instance $(x',g(p))$ of $B$
	in time $f(p) |x|^{\alpha}$,
	so that $(x,p) \in A$ if and only if $(x',g(p)) \in B$.
\end{definition}

To show hardness in the parameterized setting, it is enough to give a parameterized reduction from a known hard problem. A parameterized problem is said to be \PARANPC if it is \NPC{} even for constant values of the parameter. A classic example of a \PARANPC{} problem is graph coloring parameterized by the number of colors -- recall that it is \NPC{} to determine if a graph can be properly colored with three colors. Observe that a \PARANPC{} problem does not belong to~$XP$ unless~$\Pshort{} = \NP{}$. We are now ready to describe our contributions in greater detail. For a more detailed and formal introduction to parameterized complexity, we refer the reader to~\cite{CyganFKLMPPS15}.
